# Supplementary material for: ConsistencyPlanner: Real-time Planning with Fast-Sampling Consistency Models
Source: arXiv:2606.11569 source file (2026-06-10)
Supplement: Supplementary file 1 [file Supplementary.tex]

\clearpage
\setcounter{page}{1}
\setcounter{figure}{0}
\setcounter{table}{0}

\newcommand{\maketitlesupplementary}{
  \begin{center}
    {\LARGE \textbf{Real-Time Autonomous Driving with Consistency-Guided Multimodal Planning}}\\[1.5ex]
    % {\LARGE \textbf{Reasoning for Closed-loop Autonomous Driving}}\\[2.5ex]
    {\large Supplementary Material}\\[2ex]
  \end{center}
  \vspace{2ex}
}

\maketitlesupplementary
\appendix

\noindent We provide supplementary material to complement the main paper, arranged as follows:
\begin{itemize}
   
    \item Appendix~\ref{sup: implementation}: Implementation Details.
    \item Appendix~\ref{sup: case}: More Case Study.
    
\end{itemize}

\section{Implementation Details}
\label{sup: implementation}

\begin{table*}[!htbp]
  \centering
  \caption{\enspace Hyperparameter settings of the Training}
    \begin{tabular}{cc}
    \toprule
    Hyperparameter & Value \\
    \midrule
    Training epochs & 20 \\
    % Optimizer & AdamW \\
    Learning rate & 2e-4 \\
    Learning rate scheduler & OneCycleLR \\
    Ratio of learning rate warmup phase & 0.04 \\
    Initial learning rate divisor & 25.0 \\
    Final learning rate divisor & 100 \\
    \bottomrule
    \end{tabular}%
  \label{tab}%
\end{table*}%

During training, the sub-sequence \(\{t_m | m \in [T]\}\) differs from inference and follows the Karras boundary schedule~\cite{karras}:  
\[
t_m = \left(\epsilon^{1/\rho} + \frac{m-1}{T-1}\left(t_T^{1/\rho} - \epsilon^{1/\rho}\right)\right)^\rho,
\]  
where \(t_T\) denotes the terminal timestep, \(\epsilon\) is a small constant for numerical stability, and \(\rho\) controls the curvature of the schedule.

\begin{table*}[!htbp]
  \centering
  \caption{\enspace Hyperparameter setting for Consistency Models}
    \begin{tabular}{lc}
    \toprule
    Hyperparameter & Value \\
    \midrule
    % Number of discretization steps ($T$) & 40 \\
    % Terminal timestep ($t_{T}$) & 80.0 \\
    % Minimum noise level ($\epsilon$) & 0.002 \\
    % Schedule curvature ($\rho$) & 7.0 \\
     $T$ & 40 \\
    $t_{T}$ & 80.0 \\
    $\epsilon$ & 0.002 \\
    $\rho$ & 7.0 \\
    \bottomrule
    \end{tabular}%
  \label{tab:hyperparams}%
\end{table*}%
